# Supplementary material for: Kimera-Multi: Robust, Distributed, Dense Metric-Semantic SLAM for Multi-Robot Systems
Source: arXiv:2106.14386 source file (2021-12-17)
Supplement: Supplementary file 1 [file appendix.tex]

%!TEX root = ../main.tex

\begin{appendices}

\section{Additional Experimental Results}

\end{appendices}
